# Supplementary material for: MLSNet: A Policy Complying Multilevel Security Framework for Software Defined Networking
Source: arXiv:2009.10021 source file (2020-09-21)
Supplement: Supplementary file 1 [file appendix.tex]

\newpage
\newpage
\section{Appendix}
\label{sec:appendix}

\subsection{Nomenclature and notation}
\label{sec:nomenclature}
\vspace{-0mm}
\begin{table}[H]
	{{
		\centering
		\caption{Nomenclature and notation.}\label{tab:notation}
     	\vspace{-3mm}
		\begin{tabular}{|l|l|}
			\hline
			\bfseries Notation & \bfseries Description \\
			\hline
			$V$ & Set of vertices in network graph $G=\{V,E\}$\\
			\hline
			$E$ & Set of edges in network graph $G=\{V,E\}$\\
			\hline
			$F$ & Set of packet flows to be accommodated\\
			%$G^{(n)}=(V^{(n)}, E^{(n)})$ & supply graph at iteration $n$\\
			\hline
			$R$ & Set of matching fields in a flow rule\\
			\hline
			$A$ & Set of action fields in a flow rule\\
			\hline
			$S$ & Set of subjects\\
			\hline
			$O$ & Set of objects\\
			\hline
			$C$ & Set of security categories\\
			\hline $d^f$ & Size of flow $f \in F$\\
			\hline $\kappa_{ij}$ ($\widetilde{\kappa}_{ij}$) & Residual capacity of link $(i,j)$, $(i,j) \in E$\\
			\hline $\sigma_{i}$ & Security level of node $i$, $i \in V$\\
			%\hline $\sigma_{f}$ & Security level of flow $f$, $f \in F$\\
			\hline $\lambda^c_{i}$ & Security category $c$ at node $i$\\
			\hline $L$ & Set of labels that form the lattice\\
			\hline
		\end{tabular}
		\vspace{-0mm}
	}}
\end{table}

\vspace{-0mm}
\subsection{Output of SDNMap}
\label{sec:sdnmapoutput}
{\small
\textit{
	%\footnotesize
	\noindent
	\hspace{-1mm}1: SDNMap/python main.py 10.0.0.0/29 TCP h1-eth0 [] \newline
	2: Sending ARP request to 10.0.0.0\newline
	3: ... \newline
	4: Sending ARP request to 10.0.0.7\newline
	5: 10.0.0.1 / 00:00:00:00:00:01 received response from the following hosts: \newline
	6: \textbf{10.0.0.5 / 00:00:00:00:00:05}\newline
	7: ----------------------------\newline
	8: Use 10.0.0.5 / 00:00:00:00:00:05 for probing\newline
	9: --- Determine enforced protocols ---\newline
	10: ------- Check with TCP --------\newline
	11: Check if host at 10.0.0.5 - 00:00:00:00:00:05 is reachable with src addresses 10.0.0.1 - 00:00:00:00:00:01 with TCP on src port 64836 and dst port 36748\newline
	12: \textbf{Host is reachable via TCP!}\newline
	13: -------------------------------------------\newline
	14: ------- Check with ICMP -------\newline
	15: Check if host at 10.0.0.5 - 00:00:00:00:00:05 is reachable with src addresses 10.0.0.1 - 00:00:00:00:00:01 with ICMP\newline
	16: -------------------------------------------\newline
	17: ------- Check with UDP --------\newline
	18: Check if host at 10.0.0.5 - 00:00:00:00:00:05 is reachable with src addresses 10.0.0.1 - 00:00:00:00:00:01 with UDP on src port 64836 and dst port 36748\newline
	19: -------------------------------------------\newline
	20: \textbf{Accepted protocols}: \newline
	21: \textbf{TCP}\newline
	22: --- Determine which L2/L3 fields are enforced using TCP ---\newline
	23: ------- Check if layer 3 routing is used --------\newline
	24: Check if host at 10.0.0.5 - 00:00:00:00:00:05 is reachable with src addresses 10.0.0.205 - 00:00:00:00:00:01 from port 64836 to port 36748\newline
	25: Spoof ARP cache at 10.0.0.5 from 10.0.0.205 to 00:00:00:00:00:01\newline
	26: Check if host at 10.0.0.5 - 00:00:00:00:00:05 is reachable from 10.0.0.205 - 00:00:00:00:00:01 from port 64836 to port 36748\newline
	27: -------------------------------------------\newline
	28: ------- Check if layer 2 routing is used --------\newline
	29: Check if host at 10.0.0.5 - 00:00:00:00:00:05 is reachable with src addresses 10.0.0.1 - 00:00:00:25:12:b2 from port 64836 to port 36748\newline
	30: Spoof ARP cache at 10.0.0.5 from 10.0.0.1 to 00:00:00:25:12:b2\newline
	31: Check if host at 10.0.0.5 - 00:00:00:00:00:05 is reachable from 10.0.0.1 - 00:00:00:00:00:01 from port 64836 to port 36748\newline
	32: Spoof ARP cache at 10.0.0.5 from 10.0.0.1 to 00:00:00:00:00:01\newline
	33: -------------------------------------------\newline
	34: .....\newline
	35: ------- Reconstructed rules ---------\newline
	36: match=type:tcp,dl\_src:00:00:00:00:00:01,dl\_dst:00:00:00:00:00:05,\newline
	tp\_src:64836,tp\_dst:36748, nw\_src:10.0.0.1, nw\_dst:10.0.0.5\newline actions=output:\#OUT\_PORT\newline
	37: match=type:tcp,dl\_src:00:00:00:00:00:05, dl\_dst:00:00:00:00:00:01,
	tp\_src:36748, tp\_dst:64836, nw\_src:10.0.0.5,nw\_dst:10.0.0.1\newline actions=output:\#OUT\_PORT\newline
	38: -------------------------------------
}}
